# Supplementary material for: Bugs with Features: Vision-Based Fault-Tolerant Collective Motion Inspired by Nature
Source: arXiv:2512.22448 source file (2025-12-27)
Supplement: Supplementary file 1 [file false_positives.tex]

% requires \usepackage{adjustbox}, \usepackage{booktabs}
\begin{table}[p]
\centering
\caption{Average false positive count per cycle (mean of 50 runs). Swarm size is 40 robots.}
\label{tab:pg_fp}
\begin{tabular}{lrrrrrr}
\toprule
{} & 10-12 & 11-14 & 11-18 & 11-20 & 11-25 & 20-35 \\
\midrule
6-7 & 1.972 & 1.881 & 1.731 & 1.699 & 1.506 & 1.138 \\
7-8 & 1.893 & 1.807 & 1.660 & 1.572 & 1.466 & 1.105 \\
8-9 & 1.783 & 1.714 & 1.585 & 1.546 & 1.398 & 1.057 \\
9-10 & 1.737 & 1.678 & 1.551 & 1.488 & 1.369 & 1.036 \\
10-11 & 1.690 & 1.600 & 1.505 & 1.451 & 1.307 & 1.019 \\
11-12 & 1.648 & 1.529 & 1.464 & 1.401 & 1.284 & 0.985 \\
12-13 & 1.597 & 1.501 & 1.396 & 1.368 & 1.254 & 0.989 \\
13-14 & 1.562 & 1.463 & 1.378 & 1.319 & 1.218 & 0.965 \\
14-15 & 1.508 & 1.417 & 1.332 & 1.295 & 1.201 & 0.941 \\
\midrule
5-7 & 2.086 & 1.921 & 1.815 & 1.728 & 1.568 & 1.164 \\
6-8 & 1.962 & 1.835 & 1.717 & 1.631 & 1.479 & 1.120 \\
7-9 & 1.887 & 1.763 & 1.623 & 1.558 & 1.414 & 1.081 \\
8-10 & 1.770 & 1.681 & 1.576 & 1.514 & 1.391 & 1.047 \\
9-11 & 1.721 & 1.640 & 1.500 & 1.457 & 1.351 & 1.022 \\
10-12 & 1.646 & 1.553 & 1.487 & 1.427 & 1.305 & 1.008 \\
11-13 & 1.579 & 1.515 & 1.445 & 1.383 & 1.277 & 0.992 \\
12-14 & 1.547 & 1.473 & 1.385 & 1.327 & 1.252 & 0.965 \\
13-15 & 1.514 & 1.434 & 1.349 & 1.326 & 1.210 & 0.957 \\
\midrule
5-8 & 2.023 & 1.873 & 1.750 & 1.668 & 1.536 & 1.158 \\
6-9 & 1.922 & 1.802 & 1.681 & 1.587 & 1.487 & 1.101 \\
7-10 & 1.833 & 1.711 & 1.621 & 1.537 & 1.415 & 1.071 \\
8-11 & 1.759 & 1.648 & 1.548 & 1.476 & 1.362 & 1.036 \\
9-12 & 1.706 & 1.616 & 1.483 & 1.449 & 1.318 & 1.010 \\
10-13 & 1.659 & 1.555 & 1.453 & 1.403 & 1.290 & 0.995 \\
11-14 & 1.595 & 1.494 & 1.421 & 1.365 & 1.254 & 0.982 \\
12-15 & 1.532 & 1.464 & 1.368 & 1.338 & 1.234 & 0.954 \\
\midrule
5-9 & 1.954 & 1.859 & 1.716 & 1.630 & 1.478 & 1.108 \\
6-10 & 1.899 & 1.780 & 1.650 & 1.581 & 1.438 & 1.083 \\
7-11 & 1.818 & 1.708 & 1.573 & 1.503 & 1.378 & 1.046 \\
8-12 & 1.745 & 1.622 & 1.529 & 1.468 & 1.345 & 1.028 \\
9-13 & 1.682 & 1.567 & 1.470 & 1.431 & 1.305 & 1.010 \\
10-14 & 1.624 & 1.536 & 1.433 & 1.388 & 1.260 & 0.983 \\
11-15 & 1.562 & 1.482 & 1.398 & 1.344 & 1.243 & 0.978 \\
\midrule
5-10 & 1.938 & 1.852 & 1.685 & 1.625 & 1.474 & 1.106 \\
6-11 & 1.885 & 1.750 & 1.635 & 1.537 & 1.412 & 1.095 \\
7-12 & 1.795 & 1.673 & 1.544 & 1.500 & 1.375 & 1.041 \\
8-13 & 1.723 & 1.629 & 1.501 & 1.468 & 1.335 & 1.023 \\
9-14 & 1.662 & 1.574 & 1.455 & 1.395 & 1.288 & 1.007 \\
10-15 & 1.612 & 1.519 & 1.428 & 1.365 & 1.270 & 0.988 \\
\midrule
5-11 & 1.914 & 1.825 & 1.688 & 1.601 & 1.458 & 1.106 \\
6-12 & 1.861 & 1.723 & 1.624 & 1.550 & 1.409 & 1.067 \\
7-13 & 1.789 & 1.669 & 1.539 & 1.486 & 1.375 & 1.038 \\
8-14 & 1.722 & 1.621 & 1.519 & 1.455 & 1.324 & 1.016 \\
9-15 & 1.645 & 1.578 & 1.451 & 1.406 & 1.305 & 1.008 \\
\midrule
5-12 & 1.939 & 1.834 & 1.662 & 1.617 & 1.456 & 1.100 \\
6-13 & 1.833 & 1.731 & 1.614 & 1.550 & 1.428 & 1.074 \\
7-14 & 1.771 & 1.679 & 1.557 & 1.477 & 1.372 & 1.054 \\
8-15 & 1.728 & 1.607 & 1.504 & 1.456 & 1.313 & 1.030 \\
\midrule
5-13 & 1.949 & 1.837 & 1.679 & 1.613 & 1.461 & 1.114 \\
6-14 & 1.852 & 1.704 & 1.607 & 1.567 & 1.419 & 1.085 \\
7-15 & 1.807 & 1.660 & 1.579 & 1.491 & 1.383 & 1.061 \\
\midrule
5-14 & 1.953 & 1.819 & 1.700 & 1.623 & 1.482 & 1.142 \\
6-15 & 1.866 & 1.747 & 1.642 & 1.564 & 1.432 & 1.101 \\
\midrule
5-15 & 1.939 & 1.834 & 1.697 & 1.628 & 1.477 & 1.151 \\
\bottomrule
\end{tabular}
\end{table}
