# Supplementary material for: Bugs with Features: Vision-Based Fault-Tolerant Collective Motion Inspired by Nature
Source: arXiv:2512.22448 source file (2025-12-27)
Supplement: Supplementary file 3 [file order_wide.tex]

\begin{table}
\caption{Heatmap of Order}
\label{tab:heatmap}
\begin{tabular}{lrrrrrrrrrrrrrrrrrrrrrrrrrrrrrrrrrrrrrrrrrrrrrrrrrrrrrr}
\toprule
x & 6-7 & 7-8 & 8-9 & 9-10 & 10-11 & 11-12 & 12-13 & 13-14 & 14-15 & 5-7 & 6-8 & 7-9 & 8-10 & 9-11 & 10-12 & 11-13 & 12-14 & 13-15 & 5-8 & 6-9 & 7-10 & 8-11 & 9-12 & 10-13 & 11-14 & 12-15 & 5-9 & 6-10 & 7-11 & 8-12 & 9-13 & 10-14 & 11-15 & 5-10 & 6-11 & 7-12 & 8-13 & 9-14 & 10-15 & 5-11 & 6-12 & 7-13 & 8-14 & 9-15 & 5-12 & 6-13 & 7-14 & 8-15 & 5-13 & 6-14 & 7-15 & 5-14 & 6-15 & 5-15 \\
\midrule
10-12 & 0.809 & 0.797 & 0.773 & 0.801 & 0.822 & 0.847 & 0.813 & 0.795 & 0.767 & 0.851 & 0.825 & 0.832 & 0.804 & 0.820 & 0.800 & 0.779 & 0.806 & 0.805 & 0.815 & 0.792 & 0.795 & 0.783 & 0.849 & 0.826 & 0.827 & 0.796 & 0.788 & 0.795 & 0.823 & 0.811 & 0.832 & 0.812 & 0.819 & 0.798 & 0.831 & 0.801 & 0.810 & 0.795 & 0.833 & 0.788 & 0.818 & 0.801 & 0.802 & 0.811 & 0.793 & 0.759 & 0.787 & 0.813 & 0.813 & 0.816 & 0.837 & 0.838 & 0.801 & 0.787 \\
11-14 & 0.808 & 0.824 & 0.794 & 0.845 & 0.824 & 0.773 & 0.794 & 0.792 & 0.773 & 0.822 & 0.821 & 0.823 & 0.812 & 0.795 & 0.793 & 0.788 & 0.773 & 0.802 & 0.789 & 0.809 & 0.797 & 0.777 & 0.832 & 0.806 & 0.799 & 0.803 & 0.824 & 0.816 & 0.817 & 0.808 & 0.799 & 0.781 & 0.779 & 0.834 & 0.824 & 0.806 & 0.826 & 0.787 & 0.792 & 0.845 & 0.778 & 0.793 & 0.802 & 0.833 & 0.831 & 0.791 & 0.794 & 0.790 & 0.802 & 0.759 & 0.777 & 0.811 & 0.808 & 0.803 \\
11-18 & 0.824 & 0.793 & 0.793 & 0.807 & 0.817 & 0.805 & 0.744 & 0.762 & 0.768 & 0.858 & 0.814 & 0.799 & 0.818 & 0.794 & 0.814 & 0.813 & 0.782 & 0.762 & 0.837 & 0.817 & 0.819 & 0.804 & 0.798 & 0.782 & 0.798 & 0.792 & 0.818 & 0.819 & 0.792 & 0.823 & 0.808 & 0.804 & 0.799 & 0.805 & 0.834 & 0.750 & 0.809 & 0.769 & 0.781 & 0.823 & 0.836 & 0.782 & 0.822 & 0.775 & 0.784 & 0.785 & 0.828 & 0.781 & 0.809 & 0.790 & 0.821 & 0.810 & 0.809 & 0.788 \\
11-20 & 0.847 & 0.787 & 0.821 & 0.810 & 0.827 & 0.792 & 0.776 & 0.776 & 0.747 & 0.849 & 0.832 & 0.778 & 0.811 & 0.782 & 0.818 & 0.784 & 0.764 & 0.780 & 0.819 & 0.827 & 0.807 & 0.788 & 0.802 & 0.792 & 0.787 & 0.766 & 0.814 & 0.813 & 0.786 & 0.804 & 0.810 & 0.794 & 0.755 & 0.825 & 0.795 & 0.796 & 0.802 & 0.781 & 0.773 & 0.798 & 0.824 & 0.793 & 0.812 & 0.772 & 0.822 & 0.798 & 0.777 & 0.785 & 0.789 & 0.822 & 0.774 & 0.797 & 0.774 & 0.776 \\
11-25 & 0.813 & 0.840 & 0.796 & 0.802 & 0.767 & 0.770 & 0.746 & 0.729 & 0.682 & 0.838 & 0.815 & 0.780 & 0.807 & 0.802 & 0.784 & 0.733 & 0.746 & 0.710 & 0.848 & 0.832 & 0.822 & 0.815 & 0.773 & 0.765 & 0.760 & 0.728 & 0.782 & 0.823 & 0.773 & 0.792 & 0.782 & 0.743 & 0.741 & 0.808 & 0.797 & 0.799 & 0.784 & 0.781 & 0.763 & 0.792 & 0.796 & 0.773 & 0.778 & 0.781 & 0.759 & 0.800 & 0.748 & 0.747 & 0.789 & 0.764 & 0.759 & 0.778 & 0.743 & 0.741 \\
20-35 & 0.783 & 0.799 & 0.780 & 0.802 & 0.778 & 0.717 & 0.744 & 0.700 & 0.632 & 0.812 & 0.812 & 0.814 & 0.809 & 0.773 & 0.762 & 0.732 & 0.688 & 0.629 & 0.838 & 0.802 & 0.785 & 0.769 & 0.772 & 0.750 & 0.727 & 0.668 & 0.790 & 0.784 & 0.753 & 0.786 & 0.752 & 0.730 & 0.726 & 0.808 & 0.822 & 0.767 & 0.746 & 0.743 & 0.720 & 0.770 & 0.771 & 0.734 & 0.725 & 0.694 & 0.782 & 0.771 & 0.759 & 0.708 & 0.736 & 0.753 & 0.739 & 0.782 & 0.747 & 0.736 \\
\bottomrule
\end{tabular}
\end{table}
